# Supplementary material for: Influence Maximization in Real-World Closed Social Networks
Source: arXiv:2209.10286 source file (2022-09-21)
Supplement: Supplementary file 1 [file appendix.tex]

\appendix
